# Supplementary material for: Optimizing CNN Model Inference on CPUs
Source: arXiv:1809.02697 source file (2019-07-05)
Supplement: Supplementary file 1 [file supplementary_material.pdf]

# Optimizing CNN Model Inference on CPUs

Supplementary material

Here is how to define and schedule a convolution (CONV) operation in the way we described in Section 3.1.1. `declaration_conv_NCHWc` defines the computation of CONV in NCHW[x]c layout with necessary padding and stride setting. `schedule_conv_NCHWc` uses TVM scheduling primitives to schedule the computation as the procedure described in Algorithm 1. We used a high-level language (Python) instead of intrinsics and/or assembly codes that a high-performance implementation typically does. This allows us to try out different ideas easily, and facilitates the layout transform elimination and best optimization scheme search we introduced in Section 3.2 and 3.3.

In [ ]:
```
def declaration_conv_NCHWc(wkl, sch, data, kernel):
    """Define convolution computation in NCHW[x]c layout

    Parameters
    ----------
    wkl : namedtuple
        The CONV workload configuration

    sch : namedtuple(ic_bn, oc_bn, reg_n, unroll_ker)
        The schedule configuration

    data : tvm.Tensor
        Input feature map in NCHW[x]c layout

    kernel : tvm.Tensor
        Kernel in KCRS[x]c[y]k layout
    """
    batch_size = data.shape[0]
    # Calculate the output height and width
    out_height = (wkl.height + 2 * wkl.hpad - wkl.hkernel) // wkl.hstride + 1
    out_width = (wkl.width + 2 * wkl.wpad - wkl.wkernel) // wkl.wstride + 1

    # Pad NCHW[x]c data
    data_pad = pad(data, (0, 0, wkl.hpad, wkl.wpad, 0), name="data_pad")

    # Define the output shape
    oshape = (batch_size, wkl.out_filter//sch.oc_bn,
              out_height, out_width, sch.oc_bn)

    # Define the reduce axes
    ic = tvm.reduce_axis((0, wkl.in_filter), name="ic")
    kh = tvm.reduce_axis((0, wkl.hkernel), name="kh")
    kw = tvm.reduce_axis((0, wkl.wkernel), name="kw")

    # Define the computation in NCHW[x]c layout
    conv = tvm.compute(oshape, lambda n, oc_chunk, oh, ow, oc_block:
                       tvm.sum(data_pad[n, ic//wkl.ic_bn,
```

```python
                                              oh*wkl.hstride+kh,
                                              ow*wkl.wstride+kw,
                                              ic%wkl.ic_bn].astype(wkl.out_dtype) *
                                     kernel[oc_chunk, ic//wkl.ic_bn,
                                            kh, kw, ic%wkl.ic_bn, oc_block],
                                     axis=[ic, kh, kw]), name="conv2d_NCHWc")
    return conv


def schedule_conv_NCHWc(sch, conv):
    """Schedule the convolution in NCHW[x]c layout

    Parameters
    ----------
    sch : namedtuple(ic_bn, oc_bn, reg_n, unroll_ker)
        The schedule configuration

    conv : tvm.tensor.ComputeOp
        Compute node generated by declaration_conv_NCHWc
    """
    s = tvm.create_schedule(conv.op)
    # Create a cache stage to help codegen further promote to register.
    CC = s.cache_write(conv, 'global')

    _, oc_chunk, oh, ow, oc_block = s[conv].op.axis
    ow_chunk, ow_block = s[conv].split(ow, factor=sch.reg_n)
    s[C].reorder(oc_chunk, oh, ow_chunk, ow_block, oc_block)
    # parallel over oc_chunk and oh
    parallel_axis = s[C].fuse(oc_chunk, oh)
    s[C].parallel(parallel_axis)

    # the inner loop where CC computes,
    # i.e., ow_block was split according to the number of registers
    s[CC].compute_at(s[C], ow_chunk)
    _, oc_chunk, oh, ow, oc_block = s[CC].op.axis
    ic, kh, kw = s[CC].op.reduce_axis

    # split to keep same as that in s[conv]
    ow_chunk, ow_block = s[CC].split(ow, factor=sch.reg_n)
    ic_chunk, ic_block = s[CC].split(ic, factor=sch.ic_bn)

    s[CC].reorder(oc_chunk, oh, ow_chunk, ic_chunk, kh, kw,
                  ic_block, ow_block, oc_block)
    if sch.unroll_ker:
        s[CC].unroll(kw)
        s[CC].unroll(kh)

    # Explictily use vectorization instruction
    s[CC].vectorize(oc_block)
    # Unroll ow_block < # of registers,
    # so that it can be optimized to use registers.
    s[CC].unroll(ow_block)

    return s
```
